# Supplementary material for: Role of defects in the thermodynamic stability of grain boundary phases at asymmetric tilt boundaries in copper
Source: arXiv:2601.16611 ancillary file (2026-01-23)
Supplement: Supplementary file 1 [file supplemental-material.pdf]

# SUPPLEMENTAL MATERIAL

## Role of defects in the thermodynamic stability of grain boundary phases at asymmetric tilt boundaries in copper

Swetha Pemma,[1] Lena Langenohl,[1] Saba Saood,[1] Yoonji Choi,[1] Rebecca Janisch,[2] Christian H. Liebscher,[1,3,4] Gerhard Dehm,[1] and Tobias Brink[1]

[1]*Max Planck Institute for Sustainable Materials, Max-Planck-Straße 1, 40237 Düsseldorf, Germany*
[2]*Interdisciplinary Centre for Advanced Materials Simulation (ICAMS), Ruhr-Universität Bochum, 44780 Bochum, Germany*
[3]*Research Center Future Energy Materials and Systems, Ruhr-Universität Bochum, 44801 Bochum, Germany*
[4]*Faculty of Physics and Astronomy, Ruhr-Universität Bochum, 44801 Bochum, Germany*

### I. GRAIN BOUNDARY PHASE FRACTIONS – SUPPLEMENTAL DATA

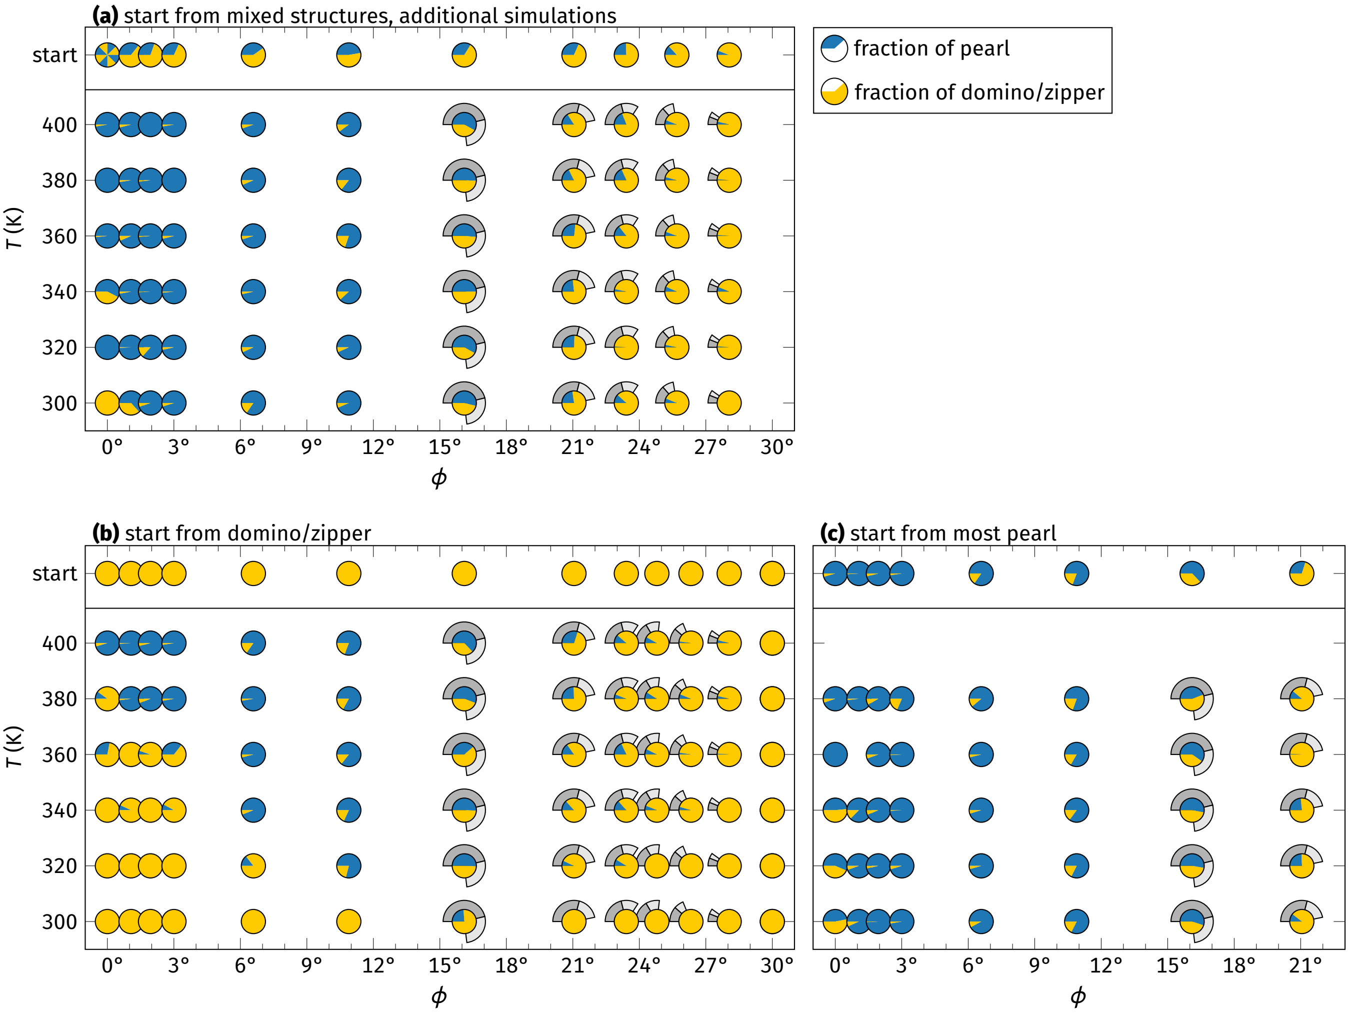


**Supplemental Fig. S1:** The GB phases present in asymmetric tilt GBs after equilibrating at temperatures between 300 K and 400 K for $t = 100\,\mathrm{ns}$. The topmost row shows the fraction of GB phases in the starting structure. Here, we present supplemental data to Fig. 5 in the main text. For each inclination and temperature, the pie chart shows the fraction of the two GB phases. Starting from 16°, there are gray bars around the data points. These indicate the maximum possible fractions of pearl phase in faceted GBs (see Sec. VIII and Fig. 13(d) in the main text). The dark gray region is for symmetric pearl facets. The light gray region indicates how much longer the pearl facets can become if they are asymmetric ($\phi = 10.89°$). (a) We show here another set of mixed structures from GRIP in addition to the one shown in Fig. 5 in the main text. The symmetric GBs at $\phi = 0°$ started from alternating domino and pearl regions of length 6 nm. In (b), simulations started from pure domino/zipper phase. (c) We then took the structures annealed at 400 K and continued annealing them at lower temperatures.

## II. DICHROMATIC PATTERN OF Σ37c [11$\bar{1}$] TILT GRAIN BOUNDARIES

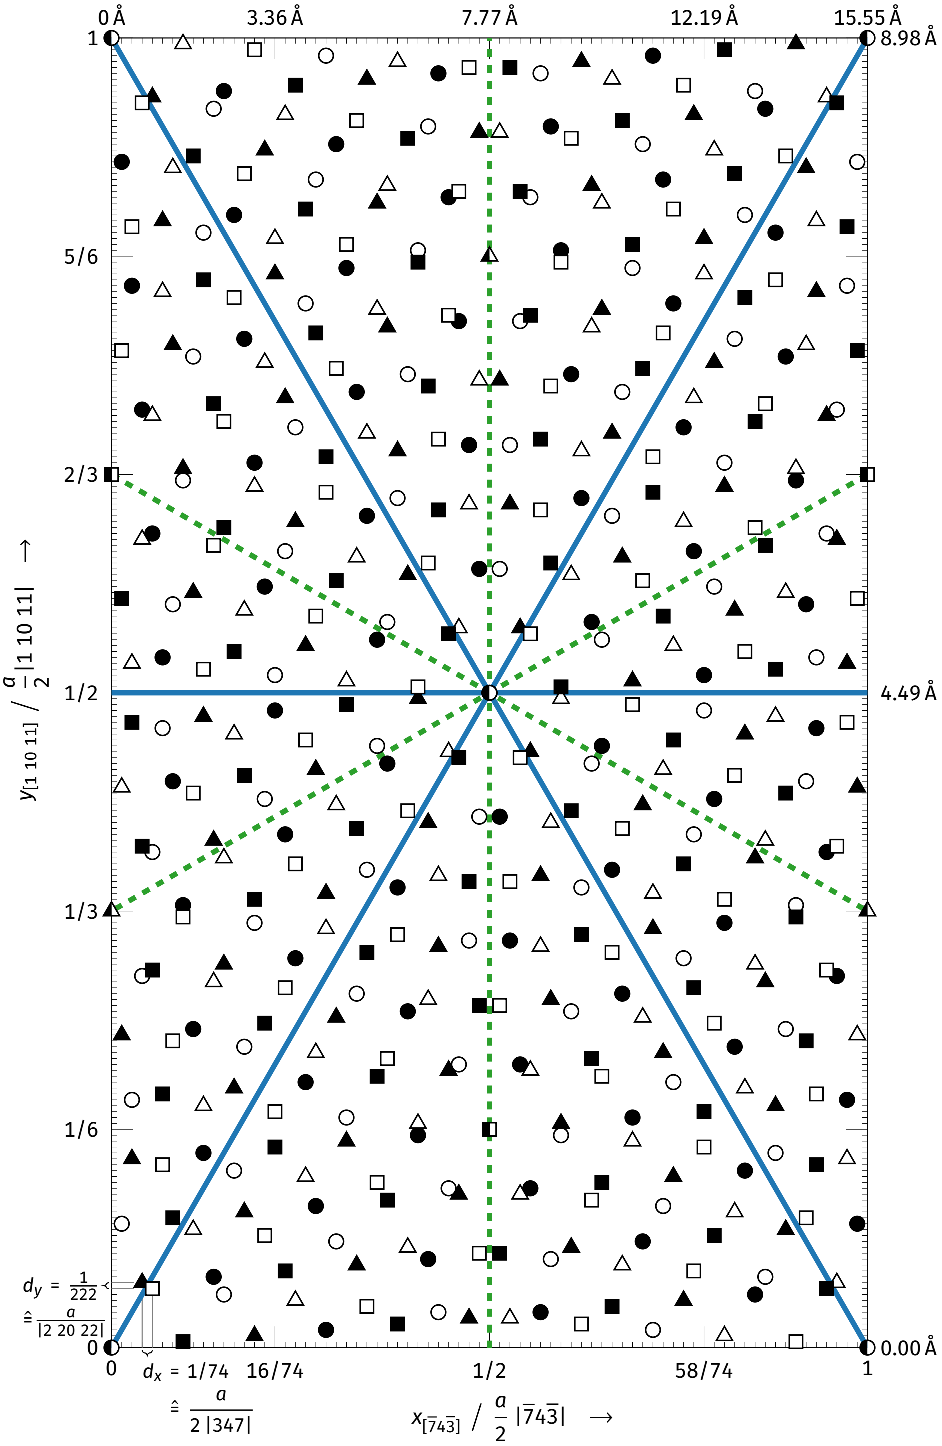


**Supplemental Fig. S2:** Full dichromatic pattern of Σ37c [11$\bar{1}$] tilt GBs. Black symbols represent the upper crystallite, white symbols the lower crystallite. Symbol shapes indicate the crystalligraphic (11$\bar{1}$) plane. The blue lines indicate the quasi-symmetric GB planes of the pearl and domino phases, while the dashed green lines represent the symmetric GB planes of the zipper phase. The pattern repeats along the vertical direction three times, but on different (11$\bar{1}$) planes.

## III. CRYSTALLOGRAPHICALLY POSSIBLE DEFECTS

We show the dichromatic patterns after shifting by various Burgers vectors **b**. Step heights and possible defect distances can be read from the shifted patterns as described for Fig. 2 in the main paper. The axes of the dichromatic patterns shown here correspond to the ones of Fig. 7 in the main paper.

Lines stand in for the migration of the GB plane due to the defect, with the orange line representing the original plane and other colors representing the new plane corresponding to a specific defect. For illustration, the planes are drawn through coincidence sites, but the results are the same for any other parallel plane.

Possible distances $r$ between defects are indicated based on the shift in $x$ direction of the circled reference points. There is an infinite set of possible distances due to the periodicity of length $74\,d_x$. The variable $n$ thus represents an arbitrary integer.

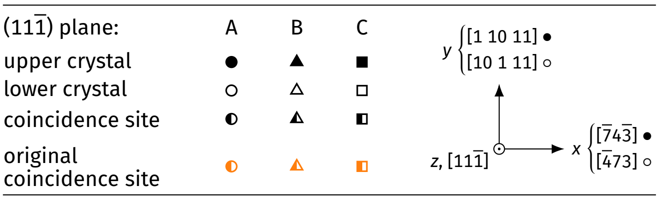


### A. Type I/II

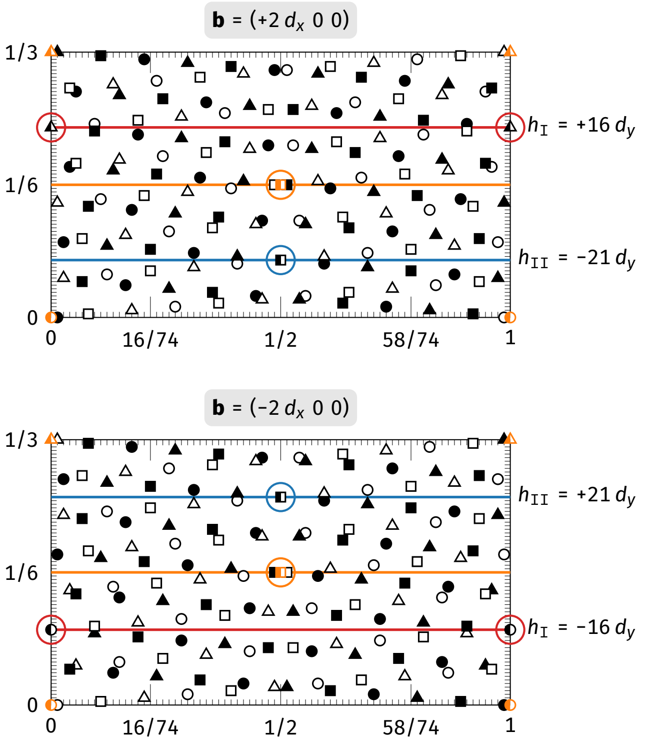


$$r_{\mathrm{I}} = |37 + 74n|\, d_x$$
$$r_{\mathrm{II}} = |\ 0 + 74n|\, d_x \quad \text{with} \quad r_{\mathrm{II}} > 0$$

### B. Type III/IV

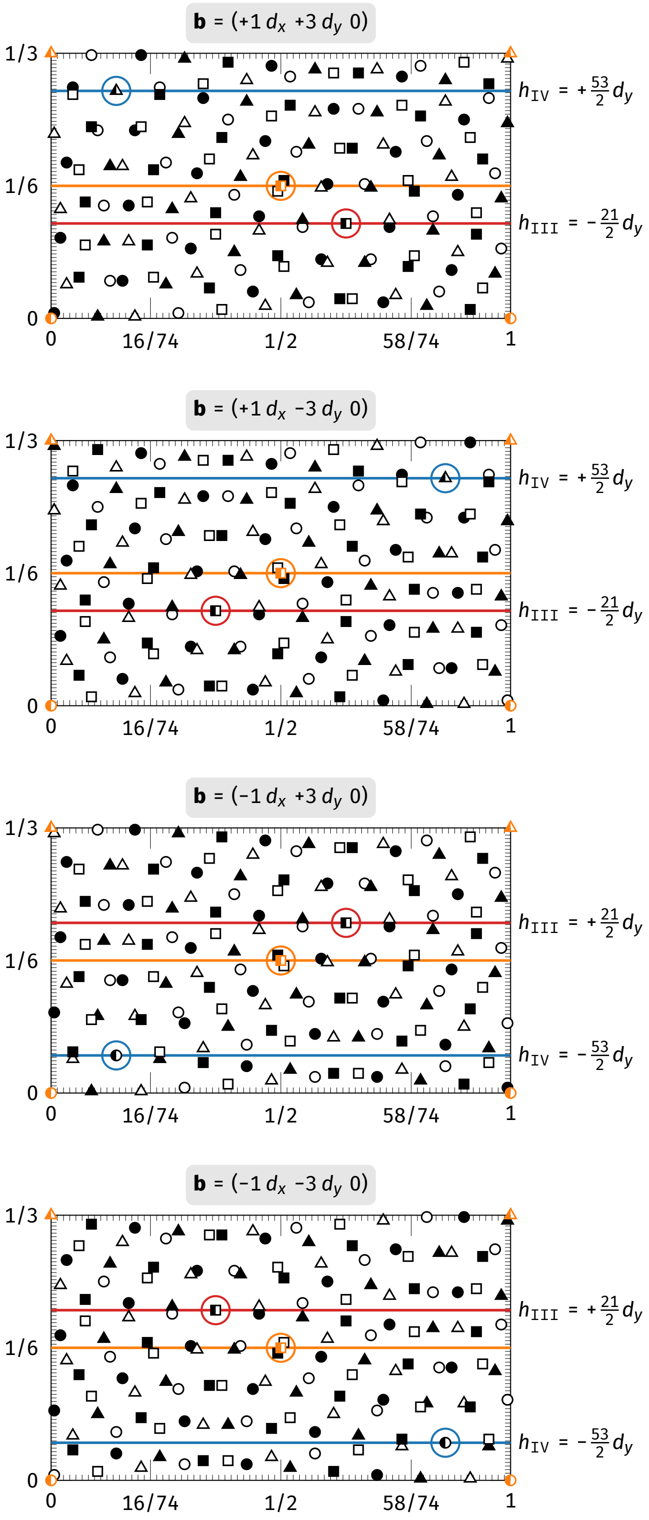


$$r_{\mathrm{III}} = \left|\frac{21}{2} + 74n\right|\, d_x$$

$$r_{\mathrm{IV}} = \left|\frac{53}{2} + 74n\right|\, d_x$$

## C. Type V

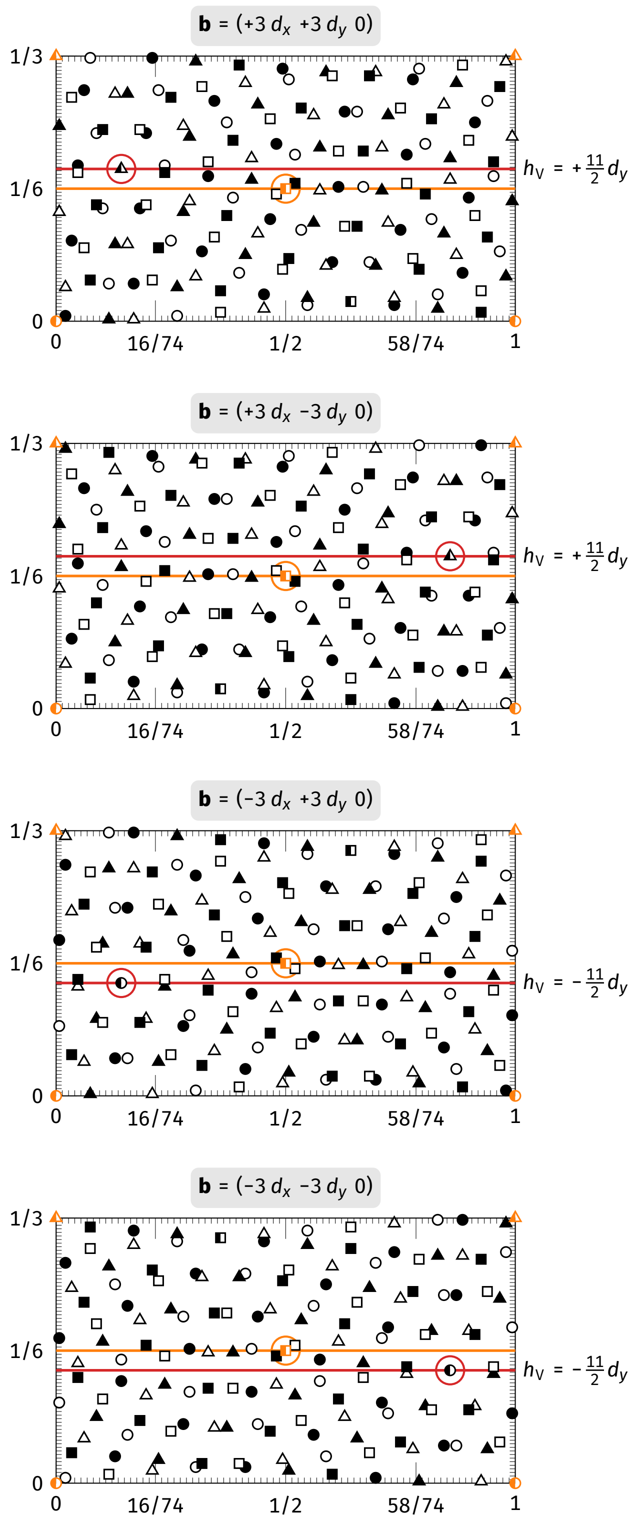


$$r_{\text{V}} = \left|\frac{53}{2} + 74n\right| d_x$$

## D. Type VI/VII

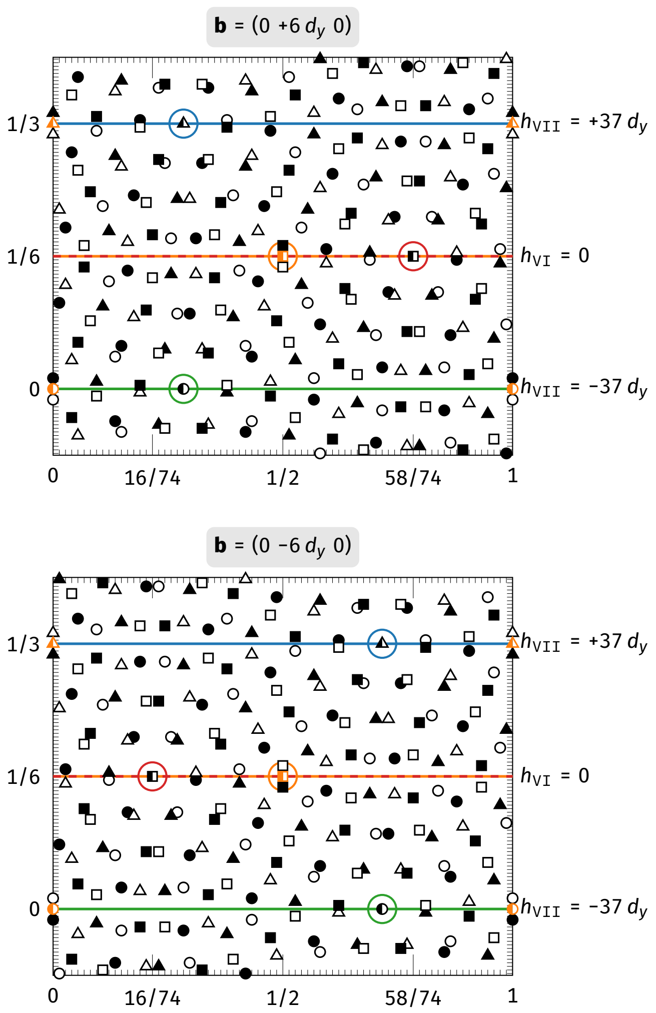


$$r_{\text{VI}} = |21 + 74n|\, d_x$$
$$r_{\text{VII}} = |16 + 74n|\, d_x$$

## E. Type VIII

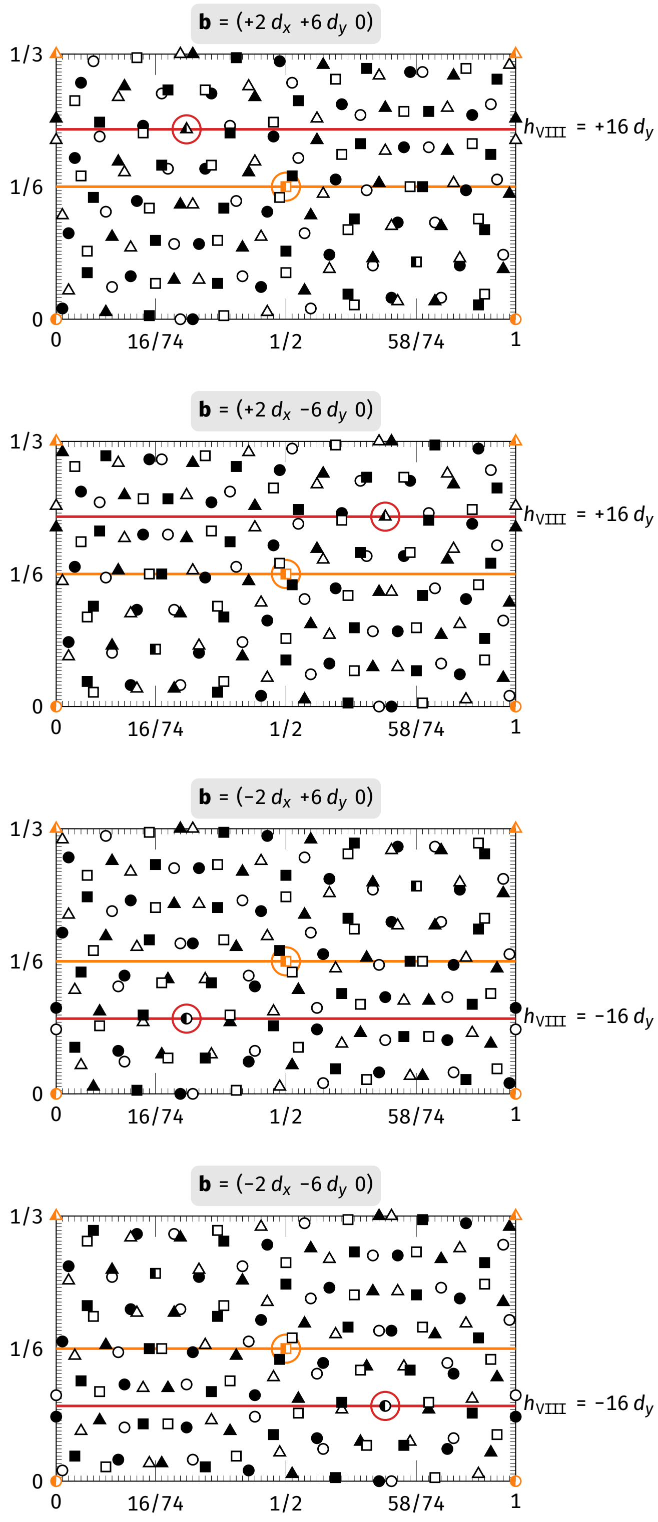


$$r_{\rm VIII} = |16 + 74n|\, d_x$$

## F. Zipper type I/T

Type "T" corresponds to the terrace defects (red circuit) in Fig. 14(a),(f) of the main text.

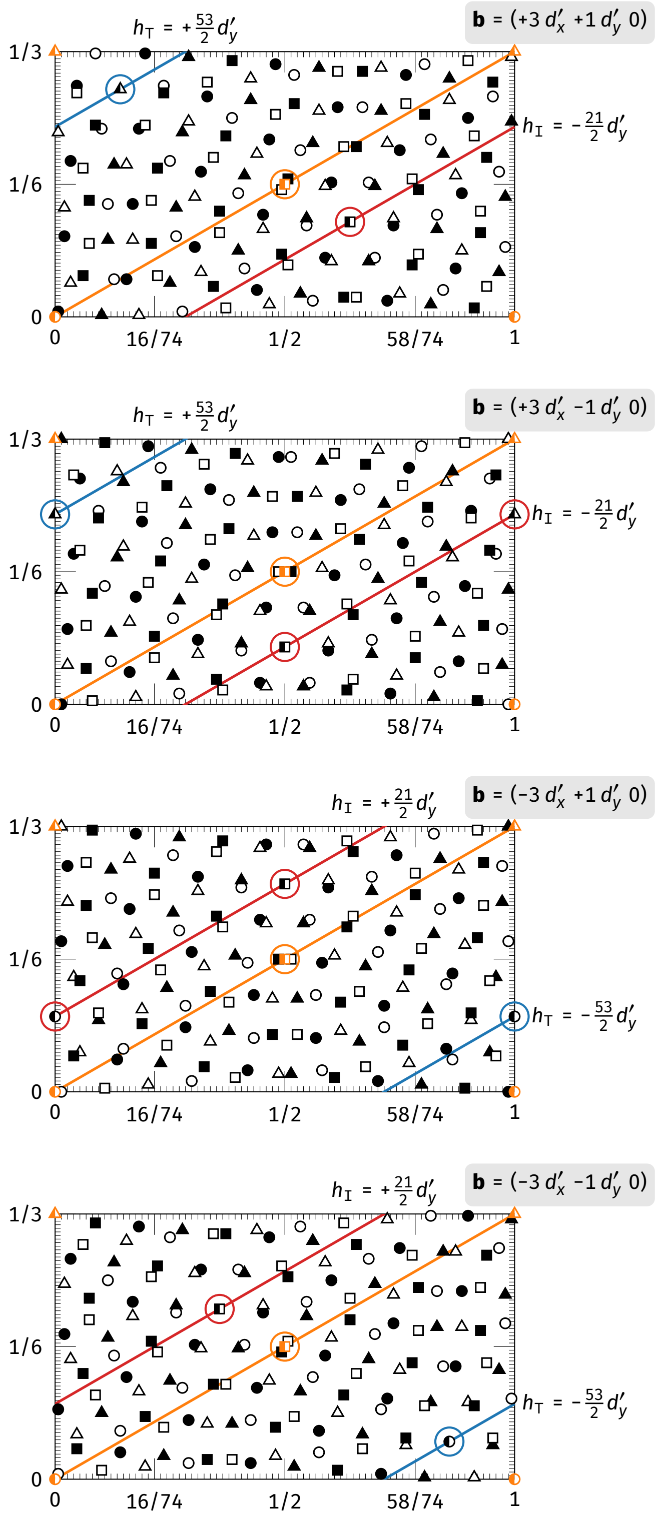


$$r_{\rm I} = \left|\frac{21}{2} + 74n\right|\, d'_x \qquad r_{\rm T} = \left|\frac{53}{2} + 74n\right|\, d'_x$$

Note that while the periodicity along the $x'$ direction of zipper is $222d'_x$, motifs are repeated every $74d'_x$, albeit on a different $(11\bar{1})$ plane. So these defect distances are allowed when there is a motif shift along $z$ (tilt axis) in the GB. This cannot be seen in the projection onto the $x'y'$ plane.

## IV. STEP ENERGIES

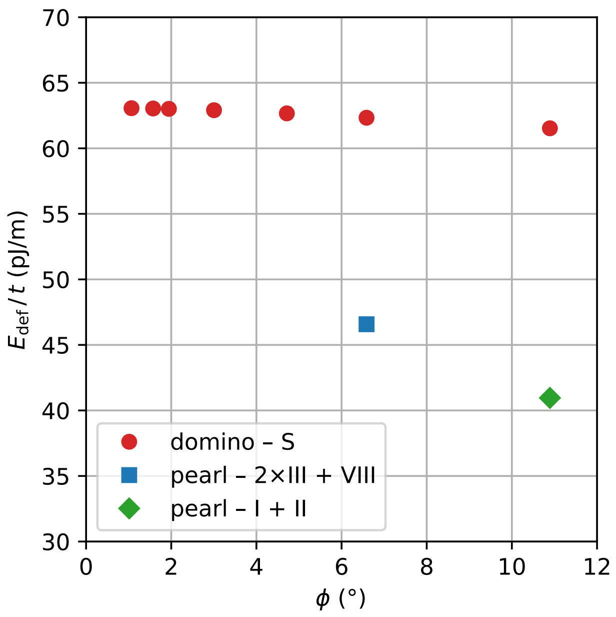


**Supplemental Fig. S3:** Defect energies of steps in domino and pearl. In domino, the step is the S defect with $n = 1$ (see Fig. 8 in the main text). To achieve different inclinations, the distance between the step defects is varied by inserting more defect-free domino unit cells in between. This is the lowest-energy configuration up to $\phi = 10.89°$, see also Fig. S7. The energy of the defect is approximately constant with $\phi$. The small variations are a result of the overlapping stress fields around the defects. For pearl, no pure steps exist, but different disconnections can be combined to achieve an overall $\mathbf{b} = \mathbf{0}$ with finite $h$.

## V. GRAIN BOUNDARY PHASE JUNCTIONS

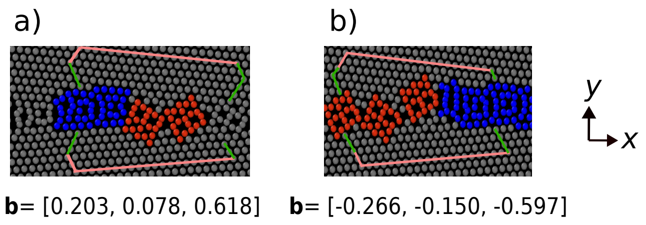


**Supplemental Fig. S4:** Analysis of two phase junctions observed in mixed pearl/domino GBs, lengths in Ångström. (a) For a simple phase junction, we find the same Burgers vector content as previously observed (Langenohl et al., Nat. Commun. **13**, 3331, 2022). In (b), there is an additional disconnection next to the junction.

## VI. STEM IMAGES

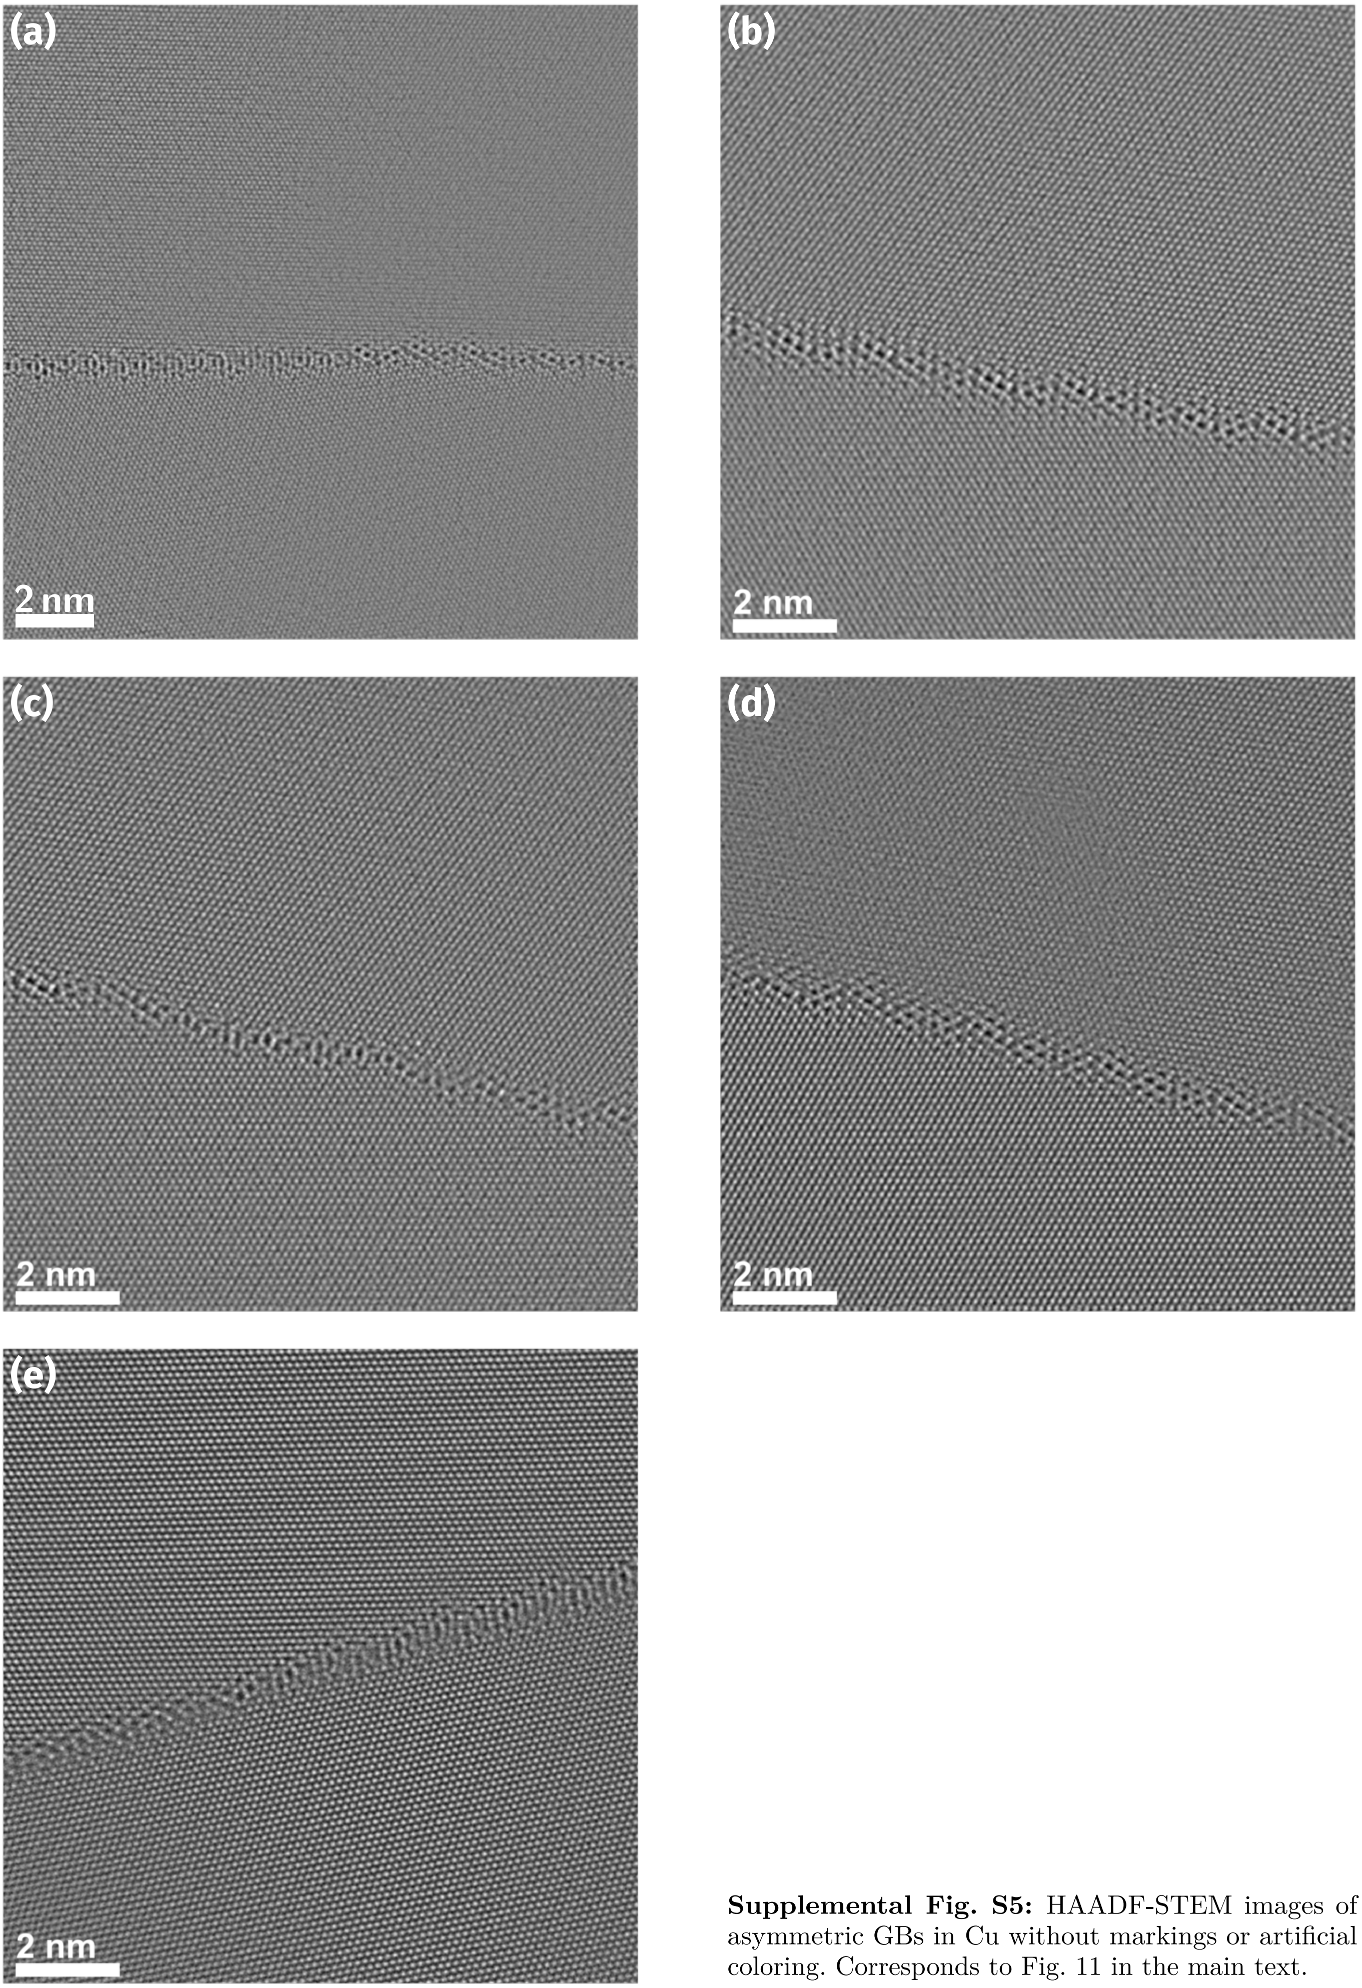


**Supplemental Fig. S5:** HAADF-STEM images of asymmetric GBs in Cu without markings or artificial coloring. Corresponds to Fig. 11 in the main text.

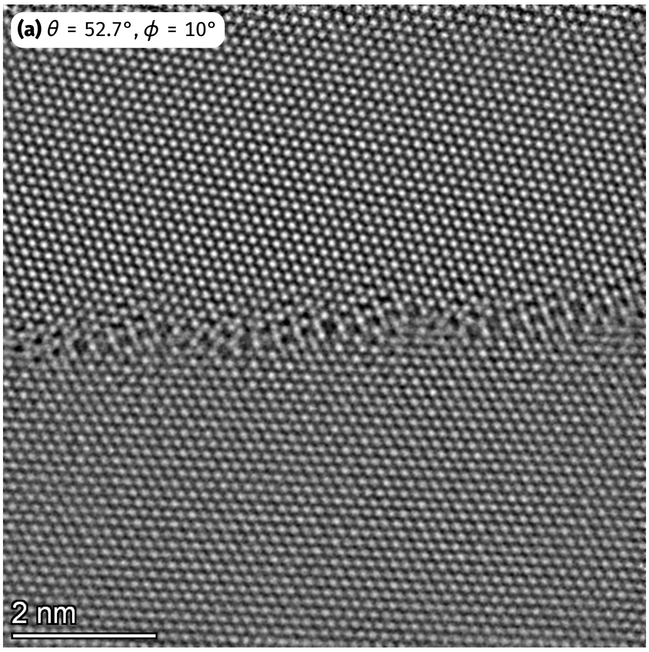


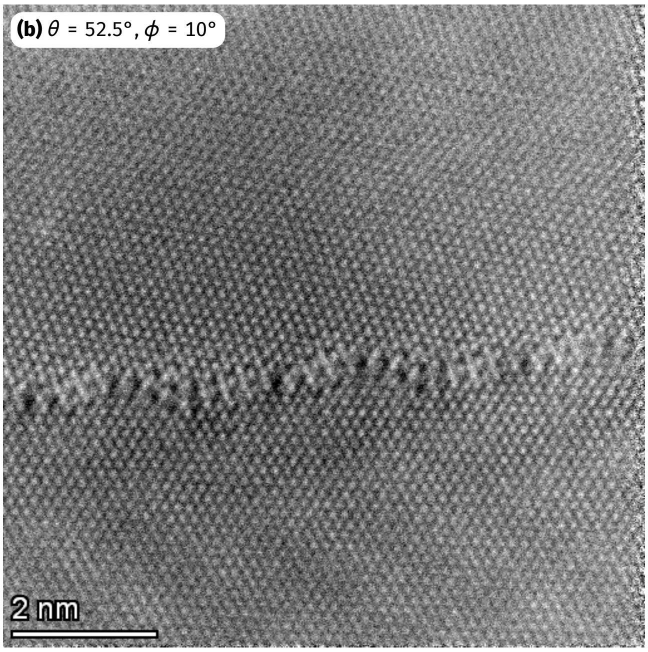


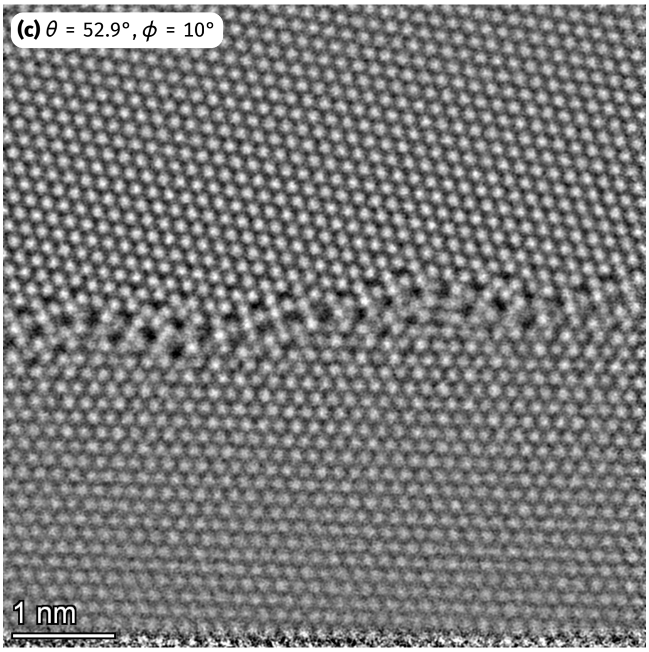


**Supplemental Fig. S6:** HAADF-STEM images of additional asymmetric GBs in Al.

## VII. DOMINO TERRACES HAVE MINIMAL SIZE

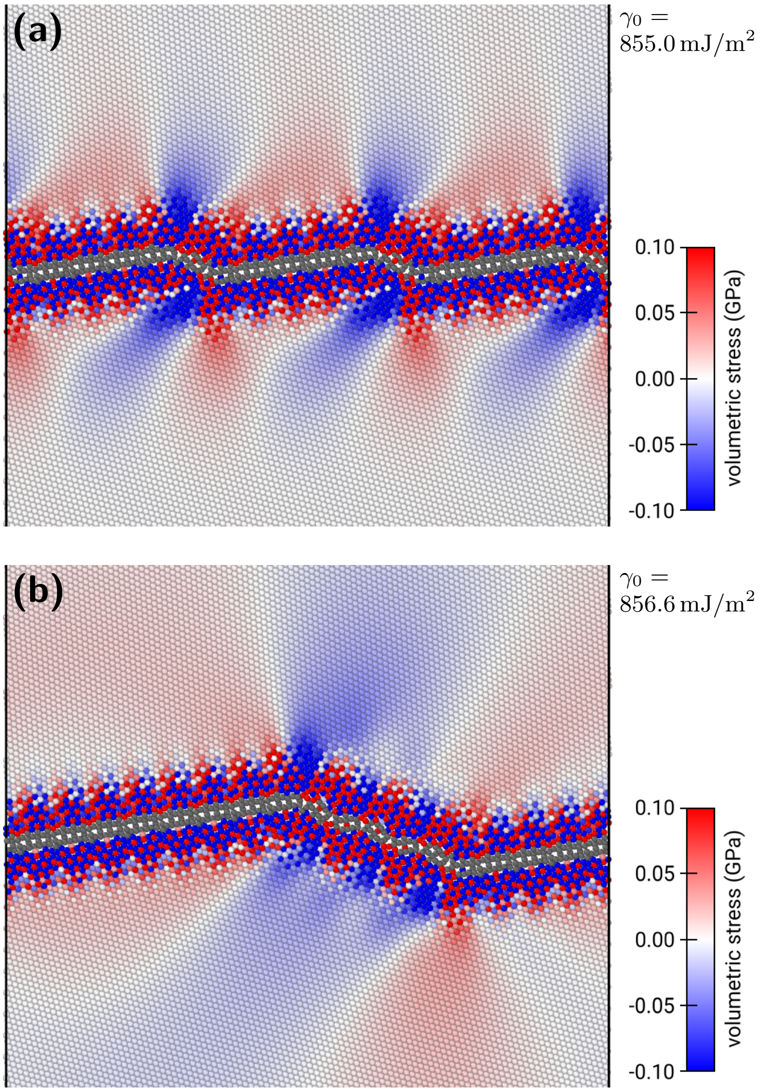


**Supplemental Fig. S7:** Asymmetric domino/zipper GBs with the same inclination. Color coding corresponds to the volumetric stress (i.e., $\mathrm{tr}(\sigma)/3$), while dark gray atoms are non-fcc atoms that belong to the GB. In (a), the step defects are individual, small steps, while in (b) there is a single domino terrace. The GB energy of the structure with individual steps is lower. This can be rationalized by looking at the stress fields: The stresses in (b) are much more long-ranging, while the small steps in (a) have more localized stresses. Thus (a) has a lower strain energy.

## VIII. FACET FRACTIONS

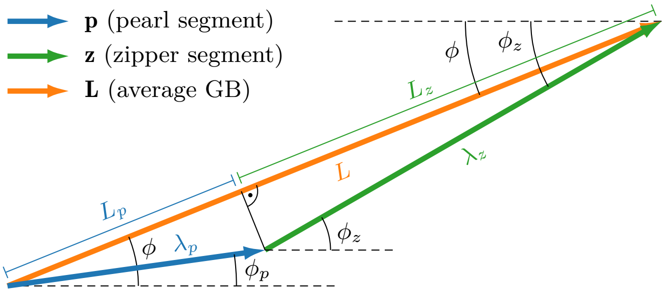


**Supplemental Fig. S8:** Periodic segment consisting of pearl and zipper facets.

We calculated the geometrically possible fractions of the different facets by assuming a periodically repeating unit of alternating pearl and zipper facets (Fig. S8).

In the projected 2D view, we describe the pearl facet $\mathbf{p}$, the zipper facet $\mathbf{z}$, and the average, periodic GB segement $\mathbf{L}$ as vectors:

$$\mathbf{p} = \lambda_p \begin{pmatrix} \cos\phi_p \\ \sin\phi_p \end{pmatrix} \qquad \mathbf{z} = \lambda_z \begin{pmatrix} \cos\phi_z \\ \sin\phi_z \end{pmatrix} \qquad \mathbf{L} = \mathbf{p} + \mathbf{z} \tag{1}$$

Since we only care about fractions of GB phases and not actual lengths, we define

$$\mathbf{L} \equiv \begin{pmatrix} \cos\phi \\ \sin\phi \end{pmatrix} \qquad \text{and thus} \qquad |\mathbf{L}| = 1. \tag{2}$$

The fraction $f_{\mathrm{pearl}}$ is defined as the relative length $L_p$ of the pearl facet projected onto the average GB plane. Thus,

$$\begin{aligned} f_{\mathrm{pearl}} &= \frac{L_p}{|\mathbf{L}|} = L_p \\ &= \mathbf{p}\cdot\mathbf{L} = \lambda_p \underbrace{(\cos\phi_p\cos\phi + \sin\phi_p\sin\phi)}_{a_p}. \end{aligned} \tag{3}$$

Equivalently,

$$\begin{aligned} f_{\mathrm{zipper}} &= \frac{L_z}{|\mathbf{L}|} = L_z \\ &= \mathbf{z}\cdot\mathbf{L} = \lambda_z \underbrace{(\cos\phi_z\cos\phi + \sin\phi_z\sin\phi)}_{a_z}. \end{aligned} \tag{4}$$

By

$$|\mathbf{L}| = 1 = L_p + L_z = \lambda_p a_p + \lambda_z a_z, \tag{5}$$

we obtain

$$\lambda_p = \frac{1-\lambda_z a_z}{a_p} \qquad \lambda_z = \frac{1-\lambda_p a_p}{a_z}. \tag{6}$$

Using only the $x$-component of $\mathbf{p}+\mathbf{z}=\mathbf{L}$, we require that

$$\lambda_p\cos\phi_p + \lambda_z\cos\phi_z = \cos\phi. \tag{7}$$

Substituting $\lambda_z$ and solving for $\lambda_p$, we find

$$\lambda_p = \frac{a_z\cos\phi - \cos\phi_z}{a_z\cos\phi_p - a_p\cos\phi_z}. \tag{8}$$

Using Eqs. 3 and 8, we can express the fractions of pearl and zipper facets only as a function of inclinations. Note that $\phi_z = 30°$, but that $\phi_p = 0°$ is only true for defect-free facets.
